# Supplementary material for: Nl2Hltl2Plan: Scaling Up Natural Language Understanding for Multi-Robots Through Hierarchical Temporal Logic Task Representation
Source: arXiv:2408.08188 source file (2024-12-05)
Supplement: Supplementary file 1 [file appendix.tex]

\section{Construction of hierarchical LTL specifications}\label{app:prompt}

\subsection{Conversion from human instructions to Hierarchical Task Tree}\label{app:conversion_htt}

% \begin{align}\label{eq:flat_task1}
%       \boxed{\text{Task} \; 1} \quad   \phi = & \, \Diamond (\apsm{furn}{1}{1} \wedge \bigcirc(\apsm{furn}{1}{1} \, \mathcal{U}\,\apsm{furn}{3}{3}))  \nonumber\\
%       & \wedge \Diamond(\apsm{pack}{3}{3} \wedge \Diamond \apsm{dock}{3}{3}) \wedge \neg \apsm{pack}{3}{3} \,\mathcal{U}\, \apsm{furn}{3}{3}  \nonumber \\
%       & \wedge \Diamond \apsm{outd}{1}{1} \wedge \Diamond \apsm{pet}{1}{1} \wedge \Diamond (\apsm{pack}{1}{1} \wedge \Diamond \apsm{dock}{1}{1}) \nonumber \\
%       & \wedge \neg \apsm{outd}{1}{1} \,\mathcal{U}\, \apsm{furn}{1}{1} \wedge \neg \apsm{outd}{1}{1} \,\mathcal{U}\, \apsm{furn}{3}{3}  \\
%       & \wedge \neg \apsm{pet}{1}{1} \,\mathcal{U}\, \apsm{furn}{1}{1} \wedge \neg \apsm{pet}{1}{1} \,\mathcal{U}\, \apsm{furn}{3}{3}  \nonumber \\
%       & \wedge \neg \apsm{pack}{1}{1} \,\mathcal{U}\, \apsm{outd}{1}{1} \wedge \neg \apsm{pack}{1}{1} \,\mathcal{U}\, \apsm{pet}{1}{1}  \nonumber \\
%       & \wedge \Diamond \apsm{heal}{2}{2} \wedge \Diamond \apsm{groc}{2}{2} \wedge  \Diamond ( \apsm{pack}{2}{2} \wedge \Diamond \apsm{dock}{2}{2} )\nonumber \\
%      & \wedge \neg \apsm{groc}{2}{2} \,\mathcal{U}\,  \apsm{heal}{2}{2} \wedge \neg \apsm{pack}{2}{2} \,\mathcal{U}\,  \apsm{groc}{2}{2} \nonumber 
% \end{align}

% \begin{figure*}[H]

% \stripsep=-10pt plus12pt minus 2pt
% \begin{strip}

\href{https://nl2hltl.github.io/prompts/Prompt_for_generating_HTT_task_decomposition.html}{Prompt for generating HTT task decomposition}
\label{fig:Prompt_for_generating_HTT_task_decomposition}

\href{https://nl2hltl.github.io/prompts/Prompt_for_HTT_sibling_relationships.html}{Prompt for extracting relationships between HTT sibling tasks}
\label{fig:Prompt_for_HTT_sibling_relationships}

\subsection{Generation of task-wise flat LTL specifications}\label{app:flat_ltl}

\href{https://nl2hltl.github.io/prompts/Prompt_for_NL2TL.html}{Nature language to LTL formula via a finetuned LLM}
\label{fig:Prompt_for_NL2TL}
% \begin{tcolorbox}[breakable,title=Nature language to LTL formula via a finetuned LLM]% \tcblower
% \textbf{Natural language description:}

% \texttt{Task\_1.1} and \texttt{Task\_1.2} can be done in any order, \texttt{Task\_1.1} and \texttt{Task\_1.2} must be completed before \texttt{Task\_1.3}, \texttt{Task\_1.3} must be completed before \texttt{Task\_1.4}.
% \tcblower
% \textbf{Possible output from the translator:}

% % {\color{red}Finally ( ( \texttt{Task\_1.1} And \texttt{Task\_1.2} ) And Finally ( \texttt{Task\_1.3} And Finally \texttt{Task\_1.4} ) )}
% Finally \texttt{Task\_1.1} And Finally \texttt{Task\_1.2} And Finally (\texttt{Task\_1.3} And Finally \texttt{Task\_1.4}) And (Not \texttt{Task\_1.3} Until \texttt{Task\_1.1}) And (Not \texttt{Task\_1.3} Until \texttt{Task\_1.2})

% \end{tcolorbox}
% \begin{figure}[H]
%     \caption{Nature language to LTL formula via a finetuned LLM}
%     \label{fig:Prompt_for_NL2TL}
% \end{figure}

\href{https://nl2hltl.github.io/prompts/Prompt_for_sequence_AP.html}{Prompt for action completion}
\label{fig:Prompt_for_sequence_AP}

\href{https://nl2hltl.github.io/prompts/complete_HLTL.html}{An example of generated hierarchical LTL specifications}
\label{fig:complete_HLTL}
% \begin{tcolorbox}[breakable, title=An example of generated hierarchical LTL specifications]
% \textbf{Task instructions:} 

% \textit{First Put the clean spatula in the drawer and put a pepper shaker in the kitchen cabinet in any order. After putting the spatula and the pepper shakers, rinse an apple to put it in the microwave. Finally, wash the spoon on the counter and place it on a plate.}
% \tcbline
% \textbf{HTT:} 
% \begin{enumerate}
% \item  {\color{blue}\verb|p0|} Perform tasks
% \begin{enumerate}
%     \item {\color{blue}\verb|p101|} Place kitchen utensils 
%     \begin{enumerate}
%         \item {\color{blue}\verb|p104|} Put the clean spatula in the drawer 
%         \item {\color{blue}\verb|p105|} put a pepper shaker in the kitchen cabinet 
%     \end{enumerate}
%     \item {\color{blue}\verb|p102|} Prepare apple for microwave 
%     \begin{enumerate}
%         \item {\color{blue}\verb|p106|} Rinse an apple and put the rinsed apple in the microwave 
%     \end{enumerate}
%     \item {\color{blue}\verb|p103|} Clean and rearrange utensils 
%     \begin{enumerate}
%         \item {\color{blue}\verb|p107|} Wash the spoon on the counter and place the washed spoon on a plate
%     \end{enumerate}
% \end{enumerate}
% \end{enumerate}

% \tcblower
% \textbf{Possible output from LLM:}
% \begin{lstlisting}[language=json]
% [
%     {
%         "p0":"<> ( p101 && ( <> ( p102 && <> p103 ) ) )"
%     },
%     {
%         "p101":"( <> p104 ) && ( <> p105 )",
%         "p102":"<> p106",
%         "p103":"<> p107"
%     },
%     {
%         "p104":"<> ( p108 && <> p109 )",
%         "p105":"<> ( p110 && <> p111 )",
%         "p106":"<> ( p112 && <> ( p113 && <> p114 ) )",
%         "p107":"<> ( p115 && <> ( p116 && <> p117 ) )"
%     },
%     {
%         "p108":[
%             "find_object_by_state(spatula, ['cleaned'])",
%             "move_to(spatula)",
%             "pickup_object(spatula)"
%             ], 
%         "p109":[
%             "move_to(drawer)",
%             "open_object(drawer)",
%             "place_object(spatula, drawer)",
%             "close_object(drawer)"
%             ],
%         "p110":[
%             "find_object_by_state(pepper_shaker, [])",
%             "move_to(pepper_shaker)",
%             "pickup_object(pepper_shaker)"
%             ],
%         "p111":[
%             "find_object_by_state(cabinet, [])",
%             "move_to(cabinet)",
%             "place_object(peppershaker, cabinet)"
%             ],
%         "p112":[
%             "find_object_by_state(apple, [])",
%             "move_to(apple)",
%             "pickup_object(apple)"
%             ],
%         "p113":[
%             "find_object_by_state(sink, [])",
%             "move_to(sink)",
%             "place_object(apple, sink)",
%             "find_object_by_state(apple, [rinsed])",
%             "pickup_object(apple)"
%             ],
%         "p114":[
%             "find_object_by_state(microwave, [])",
%             "move_to(microwave)",
%             "open_object(microwave)",
%             "place_object(apple)",
%             "close_object(microwave)"
%             ],
%         "p115":[
%             "find_object_by_state(spoon, [])",
%             "move_to(spoon)",
%             "pickup_object(spoon)"
%             ],
%         "p116":[
%             "find_object_by_state(sink, [])",
%             "move_to(sink)",
%             "place_object(spoon, sink)",
%             "pickup_object(spoon)"
%             ],
%         "p117":[
%             "find_object_by_state(plate, [])",
%             "move_to(plate)",
%             "place_object(apple,plate)"
%             ]
%     }
% ]
% \end{lstlisting}
% \end{tcolorbox}
% \begin{figure}[H]
%     \caption{An example of generated hierarchical LTL specifications.}
%     \label{fig:complete_HLTL}
% \end{figure}

\subsection{Fine-tuning LLMs to translate natural language to LTL specifications}\label{app:finetune}
Firstly, we developed a dataset comprising pairs of  natural language descriptions and their corresponding LTL formulas, subsequently fine-tuning the \verb|Mistral-7B-Instruct-v0.2|~\cite{jiang2023mistral} model for translation. Training datasets were synthesized from sources including Efficient-Eng-2-LTL~\cite{pan2023data}, Lang2LTL~\cite{liu2023lang2ltl}, nl2spec~\cite{cosler2023nl2spec}, and NL2TL~\cite{chen-etal-2023-nl2tl}. Given the domain-specific nature of these datasets, we substituted specific tasks with generic symbols such as ``\texttt{p101} should be completed before \texttt{p103}'' paired with the LTL $\pi = \Diamond ( \texttt{p101} \wedge \Diamond\, \texttt{p103})$. Next, we ask LLMs to reinterpret these ``lifted'' LTL specifications, creating a domain-agnostic dataset containing approximately 509 unique LTL formulas and 10,621 natural language descriptions produced by LLMs. Following this, the model was fine-tuned using 8-bit quantization over three epochs, achieving a translation accuracy of 98.5\% from formal language descriptions to LTL formulas.
